# Supplementary material for: Prototype Guided Backdoor Defense
Source: arXiv:2503.20925 source file (2025-03-26)
Supplement: Supplementary file 1 [file agg_cav_results_backup.tex]

\begin{table*}[t]
\caption{Results of aggregate PAV configuration on CIFAR10 compared to other configurations}
\label{tab:aggres}
\small
\begin{tabular}
{@{}L{14mm}||C{6.5mm}C{6.5mm}||C{6.5mm}C{6.5mm}|C{6.5mm}C{6.5mm}|C{6.5mm}C{6.5mm}|C{6.5mm}C{6.5mm}||C{6.5mm}C{6.5mm}|C{6.5mm}C{6.5mm}|C{6.5mm}C{6.5mm}|C{6.5mm}C{6.5mm}@{}}
%%%%%%%%%%%%%%%%%%%%%%%%%%%%%%
% \toprule[1.2pt]
\toprule[1.5pt]
% \hline
% Method  & \multicolumn{2}{c||}{Baseline} & \multicolumn{8}{c||}{Ours $T_{pro}$}     & \multicolumn{8}{c}{Ours $T_{syn}$}     \\
METHOD \faCaretRight & \multicolumn{2}{c||}{Baseline} & \multicolumn{4}{c|}{PGBD ($V^p) \quad \delta=0$} & \multicolumn{4}{c||}{PGBD ($V^p) \quad \delta=0.75$}  & \multicolumn{4}{c|}{PGBD ($V^s) \quad \delta=0$} & \multicolumn{4}{c}{PGBD ($V^s) \quad \delta=0.75$}     \\
%%%%%%%%%%%%%%%%%%%%%%%%%%%%%\hline
\hline
Agg\_PAV \faCaretRight &
  \multicolumn{2}{c||}{$\mathbf{-}$} &
  \multicolumn{2}{c|}{no agg} &
  \multicolumn{2}{c|}{agg} &
    \multicolumn{2}{c|}{no agg} &
  \multicolumn{2}{c||}{agg} &
    \multicolumn{2}{c|}{no agg} &
  \multicolumn{2}{c|}{agg} &
    \multicolumn{2}{c|}{no agg} &
  \multicolumn{2}{c}{agg} \\
% Agg\_PAV \faCaretRight &
%   \multicolumn{1}{c}{$\mathbf{-}$} &
%   \multicolumn{1}{c||}{$\mathbf{-}$} &
%   \multicolumn{1}{c}{no agg} &
%   \multicolumn{1}{c}{no agg} &
%   \multicolumn{1}{c}{agg} &
%   \multicolumn{1}{c|}{agg} &
%   \multicolumn{1}{c}{no agg} &
%   \multicolumn{1}{c}{no agg} &
%   \multicolumn{1}{c}{agg} &
%   \multicolumn{1}{c||}{agg} &
%   \multicolumn{1}{c}{no agg} &
%   \multicolumn{1}{c}{no agg} &
%   \multicolumn{1}{c}{agg} &
%   \multicolumn{1}{c|}{agg} &
%   \multicolumn{1}{c}{no agg} &
%   \multicolumn{1}{c}{no agg} &
%   \multicolumn{1}{c}{agg} &
%   \multicolumn{1}{c}{agg} \\
%%%%%%%%%%%%%%%%%%%%%%%%%%%%%%
\midrule[0.5pt]
%\midrule
ATTACK \faCaretDown & CA  & ASR  & CA & ASR & CA & ASR & CA & ASR & CA & ASR & CA & ASR & CA & ASR & CA & ASR & CA & ASR \\
%%%%%%%%%%%%%%%%%%%%%%%%%%%%%%
\midrule[1.5pt]
%\specialrule{1.5pt}{1\jot}{1\jot}
% BadNet  &              &               &    &     &    &     &    &     &    &     &    &     &    &     &    &     &    &     \\
% Trojan  &              &               &    &     &    &     &    &     &    &     &    &     &    &     &    &     &    &     \\
% Blended &              &               &    &     &    &     &    &     &    &     &    &     &    &     &    &     &    &     \\
% Signal  &              &               &    &     &    &     &    &     &    &     &    &     &    &     &    &     &    &     \\
% Wanet   &              &               &    &     &    &     &    &     &    &     &    &     &    &     &    &     &    &  \\
Badnet & 92.34 & 88.93 & 92.11 & 0.533 & 88.69 & 0.47 & 90.66 & 0.82 & 88.00 & 0.48 &  92.6 & 0.09 & 89.03 & 10.86 & 91.22 & 1.70 & 89.80 & 0.71 \\ 
Trojan & 93.00 & 100.0 & 92.17 & 90.86 & 87.20 & 74.98 & 83.60 & 6.76 & 86.22 & 37.03 & 92.18 & 99.95 & 90.34 & 4.30 & 76.34 & 2.68 & 87.18 & 17.16 \\ 
Blended & 93.06 & 92.94 & 91.33 & 5.267 & 87.23 & 4.69 & 86.11 & 4.87 & 85.44 & 12.90 & 92.27 & 74.92 & 88.58 & 39.46 & 87.51 & 2.58 & 88.10 & 25.60 \\ 
Sig & 92.90 & 89.04 & 90.72 & 0.19 & 87.13 & 2.12 & 87.18 & 0.31 & 85.80 & 0.24 & 91.58 & 71.08 & 88.10 & 3.64 & 89.94 & 7.51 & 88.93 & 0.29 \\ 
Wanet & 89.98 & 97.60 & 88.81 & 85.35 & 89.47 & 72.10 & 88.54 & 2.36 & 87.67 & 22.14 & 90.72 & 77.28 & 90.77 & 85.37 & 83.61 & 0.61 & 88.70 & 13.08 \\

%%%%%%%%%%%%%%%%%%%%%%%%%%%%%%
% \hline
\bottomrule[1.5pt]
\end{tabular}
\end{table*}


% \begin{table*}[]
% \caption{Results of aggregate cav configuration on CIFAR10 compared to other configurations}
% \begin{tabular}{@{}lllllllllllllllllll@{}}
% Attack &
%   \multicolumn{2}{l}{Baseline} &
%   \multicolumn{2}{l}{Ours (\( T_{proto}, \delta = 0\))} &
%   \multicolumn{2}{l}{Ours (\( T_{proto_{agg}}, \delta = 0\))} &
%   Ours (\( T_{proto}, \delta = 0.75\)) &
%    &
%   \multicolumn{2}{l}{Ours (\( T_{proto_{agg}}, \delta = 0.75\))} &
%   \multicolumn{2}{l}{Ours (\( T_{synth}, \delta = 0\))} &
%   \multicolumn{2}{l}{Ours (\( T_{synth_{agg}}, \delta = 0\))} &
%   Ours (\( T_{synth}, \delta = 0.75\)) &
%    &
%   \multicolumn{2}{l}{Ours (\( T_{synth_{agg}}, \delta = 0.75\))} \\
%         & CA & ASR & CA & ASR & CA & ASR & CA & ASR & CA & ASR & CA & ASR & CA & ASR & CA & ASR & CA & ASR  \\
% Badnet  & -  & -   & -  & -   & -  & -   & -  & -   & -  & -   & -  & -   & -  & -   & -  & -   & -  & -    \\
% Trojan  & -  & -   & -  & -   & -  & -   & -  & -   & -  & -   & -  & -   & -  & -   & -  & -   & -  & - \\
% Blended & -  & -   & -  & -   & -  & -   & -  & -   & -  & -   & -  & -   & -  & -   & -  & -   & -  & -    \\
% Sig     & -  & -   & -  & -   & -  & -   & -  & -   & -  & -   & -  & -   & -  & -   & -  & -   & -  & -    \\
% Wanet   & -  & -   & -  & -   & -  & -   & -  & -   & -  & -   & -  & -   & -  & -   & -  & -   & -  & -   
% \end{tabular}
% \label{tab: agg_cav_results}
% \end{table*}
